# Supplementary material for: Teaching Multiple Concepts to a Forgetful Learner
Source: arXiv:1805.08322 source file (2019-10-25)
Supplement: Supplementary file 1 [file 9_appendix_exp.tex]

% !TEX root = main.tex
%%%%%%%%%%%%%%%%%%%%%%%%%%%%%%%%%%%%%%%%%%%%%%%%%%%%%%%%%
\section{Appendix for Experiments}
..\\
..\\
..\\
..\\
..\\
..\\
..\\
..\\
..\\
..\\
..\\

\begin{figure}[!t]
  \centering
  \begin{subfigure}[b]{.3\textwidth}
    {
      \includegraphics[trim={0pt 10pt 0pt 0pt}, width=\textwidth]{./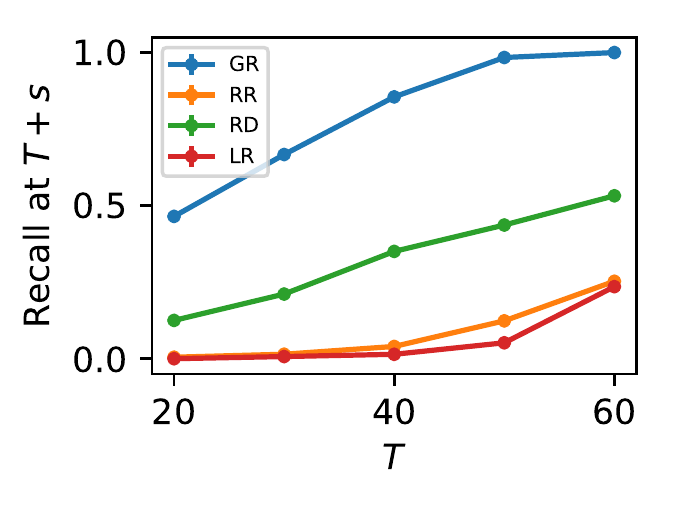}
      \caption{Recall at $T+s$ vs. T}
      \label{fig:app:recall_vs_T}
    }
  \end{subfigure}
  \begin{subfigure}[b]{.3\textwidth}
    {
      \includegraphics[trim={0pt 10pt 0pt 0pt}, width=\textwidth]{./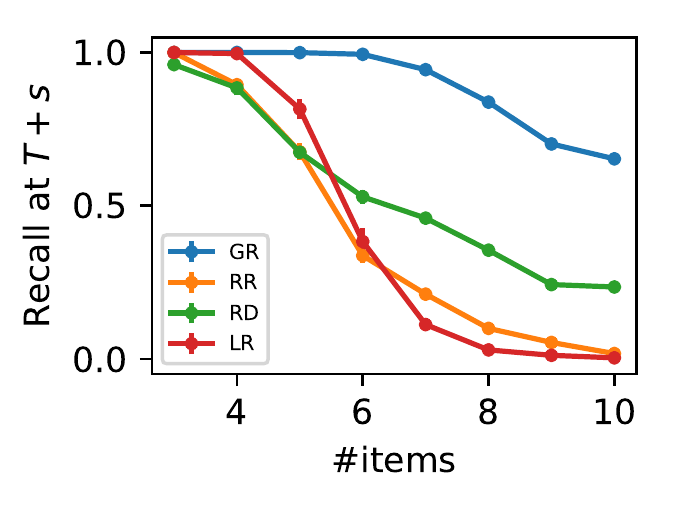}
      \caption{Recall at $T+s$ vs. m}
      \label{fig:app:recall_vs_m}
    }
  \end{subfigure}
  \begin{subfigure}[b]{.3\textwidth}
    {
      \includegraphics[trim={0pt 10pt 0pt 0pt}, width=\textwidth]{./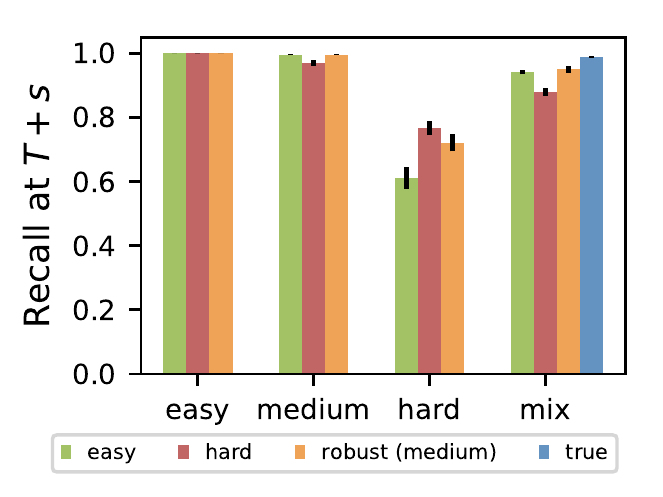}
      \caption{Robustness: Recall}
      \label{fig:app:recall_vs_c}
    }
  \end{subfigure}
  \caption{Simulated results. Evaluation metric: recall probability at $T+s$, where $s=30$.}\label{fig:app:recall_simulation}
\end{figure}

% \begin{figure}[!t]
%   \centering
%   % \begin{subfigure}[b]{0.3\textwidth}
%   %   {
%   %   \includegraphics[width=\textwidth]{./fig/empbounds/empirical_bounds_T_5_20_35_50_65_p_easy_medium_hard.pdf}
%   %   \caption{Greedy empirical bounds}
%   %   \label{fig:}
%   % }
%   % \end{subfigure}
%   \includegraphics[width=.4\textwidth]{./fig/empbounds/empirical_bounds_T_5_20_35_50_65_p_easy_medium_hard.pdf}
%   % \begin{subfigure}[b]{0.24\textwidth}
%   %   {
%   %   \includegraphics[width=\textwidth]{./fig/optimalseq_T_12_p_p3_p5_p7}
%   %   \caption{Optimal}
%   %   \label{fig:}
%   % }
%   % \end{subfigure}
%   \caption{Greedy empirical bounds}
%   \label{fig:algorithms:empirical-bounds-largeT}
% \end{figure}

\clearpage
%%%%%%%%%%%%%%%%%%%%%%%% Supplemental experiments %%%%%%%%%%%%%%%%%%%%%%
\begin{figure}[!t]
  \centering
  \begin{subfigure}[b]{.3\textwidth}
    {
      \includegraphics[trim={0pt 10pt 0pt 0pt}, width=\textwidth]{./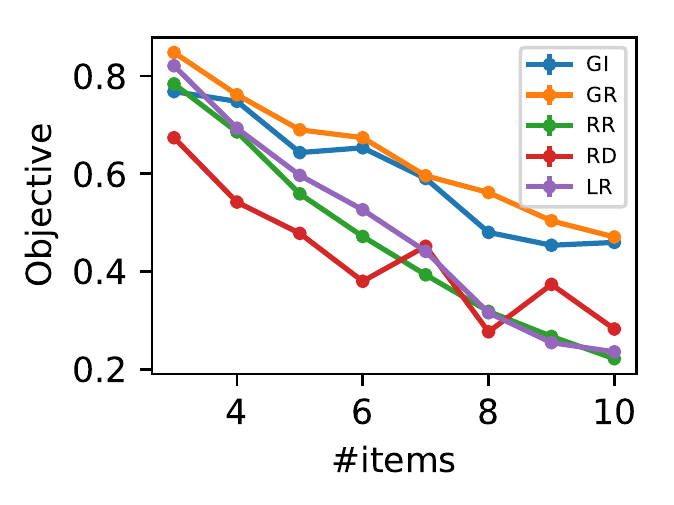}
      \caption{Objective vs. T}
      % \label{fig:obj_vs_T}
    }
  \end{subfigure}
  \begin{subfigure}[b]{.3\textwidth}
    {
      \includegraphics[trim={0pt 10pt 0pt 0pt}, width=\textwidth]{./fig/simulation/obj_vs_T__m_10_theta_3_easy_4_medium_3_hard_trial_1_interleave.pdf}
      \caption{Objective vs. m}
      % \label{fig:app:new:obj_vs_m}
    }
  \end{subfigure}
  \begin{subfigure}[b]{.3\textwidth}
    {
      \includegraphics[trim={0pt 10pt 0pt 0pt}, width=\textwidth]
      {./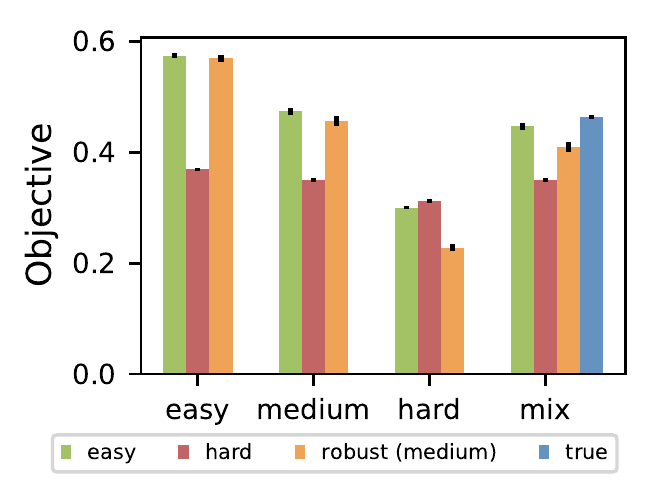}
      \caption{Robustness: Objective}
      % \label{fig:app:new:recall_vs_abratio}
    }
  \end{subfigure}
  \begin{subfigure}[b]{.3\textwidth}
    {
      \includegraphics[trim={0pt 10pt 0pt 0pt}, width=\textwidth]{./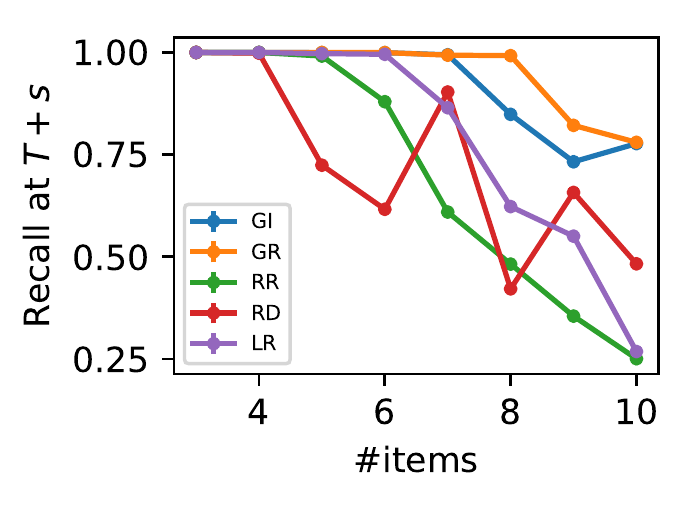}
      \caption{Recall at $T+s$ vs. T}
      \label{}
    }
  \end{subfigure}
  \begin{subfigure}[b]{.3\textwidth}
    {
      \includegraphics[trim={0pt 10pt 0pt 0pt}, width=\textwidth]{./fig/simulation/rec_vs_T__m_10_theta_3_easy_4_medium_3_hard_trial_1_interleave.pdf}
      \caption{Recall at $T+s$ vs. m}
      \label{}
    }
  \end{subfigure}
  \begin{subfigure}[b]{.3\textwidth}
    {
      \includegraphics[trim={0pt 10pt 0pt 0pt}, width=\textwidth]{./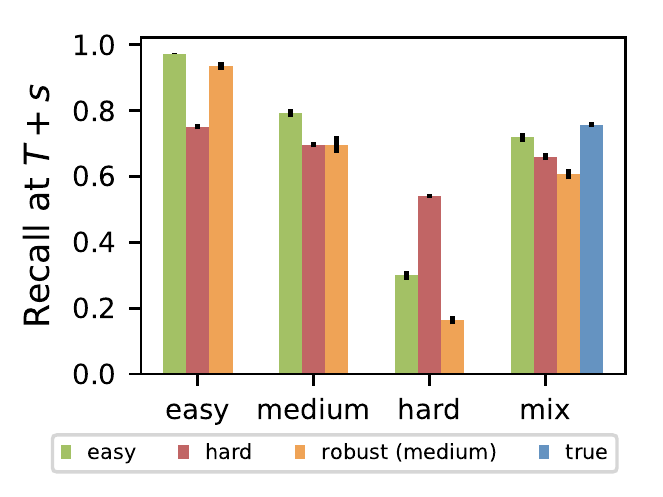}
      \caption{Robustness: Recall at T+10}
      \label{}
    }
  \end{subfigure}
  \begin{subfigure}[b]{.92\textwidth}
    {

      \includegraphics[trim={0pt 15pt 0pt 0pt},
      width=\textwidth]{./fig/simulation/obj__T_30_m_10_trials_1_mix_greedynormal.pdf}
      \caption{Greedy normal}
      \label{}
    }
  \end{subfigure}
  \begin{subfigure}[b]{.92\textwidth}
    {
      \includegraphics[trim={0pt 15pt 0pt 0pt}, width=\textwidth]{./fig/simulation/obj__T_30_m_10_trials_1_mix_greedyinterleave.pdf}
      \caption{Greedy interleave}
      \label{}
    }
  \end{subfigure}
  \begin{subfigure}[b]{0.92\textwidth}
    \centering
    {
      \includegraphics[trim={0pt 22pt 0pt 0pt}, width=\textwidth]{./fig/simulation/obj__T_30_m_10_trials_1_mix_nonadaptive.pdf}
      \includegraphics[trim={0pt 15pt 0pt 12pt}, width=\textwidth]{./fig/simulation/obj__T_30_m_10_trials_1_mix_adaptive.pdf}
      \caption{Example non-adaptive (top) and adaptive (bottom) greedy teaching sequence with $T=30, m=10$.}
      % $\theta=(2.0, 2.0, 0.0)$, $\theta=(6.0, 2.0, 0.0)$
      \label{}
    }
  \end{subfigure}
  \caption{Simulated results. }
\end{figure}

\clearpage
\begin{itemize}
\item \figref{fig:appendix:snapshots}: Snaphots for German / Birds interface
\item \figref{fig:appendix:german_histogram}: histogram for user performance
  \begin{itemize}
  \item Pick Greedy and Random. Fix m
  \item X-axis is amount of improvement: [-m, m]
  \item Y-axis is $\%$ of users with x improvement
  \end{itemize}

\item \figref{fig:appendix:birds_histogram}: Same for Birds
\end{itemize}

\begin{figure}[!t]
  \centering
  \includegraphics[width=\textwidth]{./fig/empty.png}
  \caption{Snaphots for German / Birds interface}
  \label{fig:appendix:snapshots}
\end{figure}
\begin{figure}[!t]
  \centering
  \includegraphics[width=\textwidth]{./fig/empty.png}
  \caption{histogram for user performance on German}
  \label{fig:appendix:german_histogram}
\end{figure}
\begin{figure}[!t]
  \centering
  \includegraphics[width=\textwidth]{./fig/empty.png}
  \caption{histogram for user performance on Birds}
  \label{fig:appendix:birds_histogram}
\end{figure}

%%% Local Variables:
%%% mode: latex
%%% TeX-master: "main"
%%% End:
