# Supplementary material for: Teaching Multiple Concepts to a Forgetful Learner
Source: arXiv:1805.08322 source file (2019-10-25)
Supplement: Supplementary file 2 [file 9_appendix_objective.tex]

% !TEX root = main.tex
%%%%%%%%%%%%%%%%%%%%%%%%%%%%%%%%%%%%%%%%%%%%%%%%%%%%%%%%%
\section{The Teaching Model}\label{app:teachingmodel}
\subsection{The teaching objective}
\begin{figure*}[h!]
  \centering
  \begin{subfigure}[b]{0.24\textwidth}
    {
      \includegraphics[trim={0pt 15pt 0pt 0pt}, width=\textwidth]{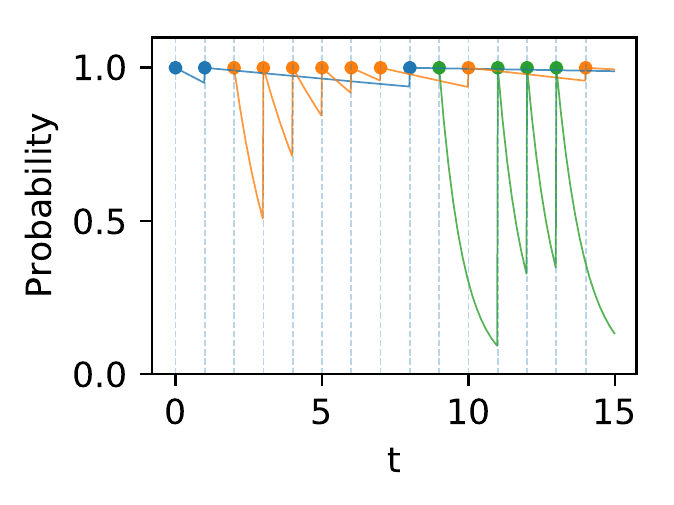}
      \caption{Greedy}
      \label{fig:objective-illu}
    }
  \end{subfigure}
  \vspace{2mm}
  \caption{Illustration of objective function
  }
  \label{fig:objective-illustration}
  % \vspace{-3mm}
\end{figure*}

%\section{Objective Function Explained}\label{app:objective}
